# Supplementary material for: Multidimensional integration through Markovian sampling under steered function morphing: a physical guise from statistical mechanics
Source: arXiv:1410.2810 ancillary file (2014-10-10)
Supplement: Supplementary file 1 [file JEMDI_SI.pdf]

# Multidimensional integration through Markovian sampling under steered function morphing: a physical guise from statistical mechanics

# SUPPLEMENTARY MATERIAL

Mirco Zerbetto and Diego Frezzato

Dipartimento di Scienze Chimiche, Università degli Studi di Padova,
via Marzolo 1, I-35131, Padova, Italy

## 1. Computational issues

In what follows we shall briefly discuss the current implementation of the integration method in the JEMDI routine, version v1.0 freely available at www.chimica.unipd.it/licc/software.html. For usage examples please see the documentary file. Numerical tests presented here and in the main text have been performed with such a basic setup.

### *1.1. Random numbers*

Uniformly distributed random numbers are generated in several parts of a single run, namely:

1) to make the unbiased sampling of the integration domain (initial not morphed "flat" state);

2) to generate Metropolis "importance sampling" Monte Carlo (IS-MC) moves in Markovian explorations of the domain (both in the preliminary exploration to achieve a trial estimate of the integral, see below, and in the sampling under function morphing if the IS-MC propagator is chosen);

3) to generate white-noise sources if the Langevin propagator is applied during morphing.

When using software random numbers generators (RNG's), careful attention must be posed on the algorithm producing the sequence of pseudo random numbers. Low quality of the algorithm can influence the results introducing important biases. With quality we intend both the ability of the algorithm of producing statistically independent sequences of random numbers, and of having long periods. The former requirement is necessary to produce a noise as much as possible white. The second one follows from the fact that the order of $N \times N_{tr} \times N_{\mathrm{steps}}$ random numbers are required. The standard C++ math library provides a linear congruential generator (LCG) to produce sequences of random numbers. LCG's are very fast (and simple to implement), but suffer of serial correlation and yield periods too short with respect to the needs in the application that we are presenting. Specially the statistical correlations among the sequence of numbers generated from a given seed make the exploration of high-dimensional spaces inefficient [1]. Thus, it is important to employ a specialized routine. Among available RNG's we selected the SPRNG (Scalable Parallel Pseudo Number Generator) v1.0 library [2]. It provides different algorithms for the generation of high quality uniformly distributed random numbers with periods at least 10 orders of magnitude longer than the standard LCG's. Moreover, the library provides methods to generate a large number of distinct streams of random numbers, which is a feature that fits our needs in a parallel run [3]. To improve the "whiteness" of the noise on each coordinate we use the feature of the SPRNG library to define $N$ different streams of pseudo random numbers, one per coordinate. Moreover, we recall that uncertainty on the integral estimate is evaluated from $M$ estimates made on equal size subsets of $N_{tr,b} = N_{tr}/M$ trajectories (see section 2.4 of the main text); in order to make each of the $M$ evaluations as much uncorrelated as possible, we reset the seed of all the streams at each repetition. The sequence of $M$ seeds is produced using the the C++ rand() function.

When using the Langevin propagator, white noise is required. Usually (this is mainly inherited by original applications in physical contexts) a Gaussian noise is employed with zero mean and unit variance. We tested two different methods to produce pseudo random numbers that are distributed over the Gaussian probability function. The former, direct method, is the inverse transform sampling, which requires the evaluation of the quantile of the Gaussian distribution [4]. The second method is the Box-Muller transform [5] which is a faster (even if not the fastest) algorithm. In place of the Gaussian distribution we tested also the noise generation using a step function. The random variable, $n$, with zero mean and unit variance, was created by collecting $R$ ($> 20$) uniformly distributed random numbers $[u_1, u_2, \ldots, u_R]$ in the range [0,1) and then applying $n = \left(\sum_{j=1}^{R} u_j - R/2\right) \sqrt{12/R}$ [6]. In our tests we empirically noticed that the Box-Muller transform is the one that performs better in terms of accuracy of the final results and computational time. Thus we decided to keep this method in the present implementation.

**Remark**. The initial seed was set equal to 6546097 in all numerical tests presented here and in the main text. This seed is given to the C++ rand() function, which is used to generate $M$ uniformly distributed pseudo random numbers between 0 and the value of the RAND_MAX constant (which is library-dependent but is at least 32767). These random numbers are used as seeds in the random numbers generator of the SPRNG library. When starting the generation of each subset of $N_{tr,b}$ trajectories, the streams of pseudo random numbers are reset with a new seed.

### *1.2. Automatic choice of best simulation parameters*

The setup of a calculation may require the intervention of the user really on many parameters. A default choice or automatic selection of most parameters can facilitate the usage of JEMDI.

A first point is the choice of the reference state, i.e. the starting level of the function morphing. As discussed in the main text, the simplest route is the morphing from an initial constant function. We implemented an automatic selection of such a constant value as follows. A preliminary IS-MC run with

$10^5$ steps is performed (optimal maximum jump-lengths per each dimension, $\delta_{\max,i}$, are determined as described below). This yields a rough estimation of the integral, $E_{trial}$. The flat reference state, $u_0(\boldsymbol{x}) = c$, is then set by $c = \ln(V_I/E_{trial})$. The advantage of employing this procedure stems in keeping the morphing factor $\Phi(\boldsymbol{\Lambda}, \boldsymbol{\Lambda}_0)$ of the order of 1, a fact that contributes to keep the numerical stability of the results during the calculation.

If the IS-MC propagator is adopted to explore the integration domain during morphing, the best $\delta_{\max,i}$ are automatically searched as follows. For simplicity we define $\delta_{\max,i} = \alpha L_i$ where $L_i$ is the extension of the $i$-th integration interval, and $\alpha$ is a single parameter which is optimized starting from $\alpha = \max_i\{L_i\}/100$ and reduced until the average acceptance percentage is above 50%. The user can lower such a threshold; we have noticed that accurate integrations can be generally performed for average acceptance percentage of moves greater than 30%.

If the Langevin propagator is employed to generate the trajectories, JEMDI is presently developed at the basic level by applying a point- and time-independent isotropic "diffusion matrix". With reference to equation 6 of the main text, this means to reduce $\mathbf{D}(\mathbf{x}, \boldsymbol{\Lambda})$ to $D\mathbf{1}$ being $\mathbf{1}$ the $N \times N$ identity matrix and $D$ a unique "diffusion coefficient" to be supplied. The user should provide, together with the integrand function, also the way to calculate the first derivatives of the natural logarithm of $f(\boldsymbol{x})$ with respect to the integration coordinates (i.e., the deterministic pseudo-forces in equation 6 of the main text). In JEMDI the user has the possibility to implement the analytical expression of the forces, which will be passed as a further argument in calling the library. If an analytical expression is not available for the derivatives, the program employs the central difference formula with increment $\delta x_i = 10^{-12}\sqrt{D\delta\hat{t}}$ for the $i$-th variable.

Another parameter to be chosen is the value of $\epsilon$ in the integration of functions with zeros and possible sign change within the integration domain; the initial value is set to $10^{-5}$. During the explorative trajectories for determining the constant $c$, a check is made to verify if $\epsilon$ is sufficiently small,

i.e. if $\epsilon << |f(\boldsymbol{x})|$. This condition is then continuously checked during the calculation; if it is not verified, the integration is stopped, $\epsilon$ is lowered, and the calculation is restarted with the new value.

*1.3. Handling of simulation consistency*

Several kinds of internal checks are implemented in the algorithm to face problematic behaviors of the code or provide to the user some information about convergence of the calculation and to which extent the final result is significant. The first important check pertains to the necessity to bound the coordinates within the integration domain. We apply reflective conditions at the boundaries of the hyper-rectangle: once the next value of a coordinate $x_i$ is computed, if it crosses the lower, $x_i^{(L)}$, or the upper, $x_i^{(U)}$, boundaries, the following correction is applied:

$$x_{i,corr} = \begin{cases} x_i + 2\left(x_i^{(L)} - x_i\right) & , \text{ if } x_i < x_i^{(L)} \\ x_i + 2\left(x_i^{(U)} - x_i\right) & , \text{ if } x_i > x_i^{(U)} \end{cases} \tag{1}$$

The reflection is continued until $x_{i,corr}$ falls inside the range of integration.

A second internal check is on possible function divergences inside the integration domain. Our tests revealed that the calculation is inaccurate if the integrand function presents singular points of divergence *inside* the integration domain, even if the integral is known to be finite. For example, the integral $\int_{-2}^{3} dx\, x^{-1}$ is finite by compensation effects but our algorithm is unable to provide the correct result due to errors in the summation of large numbers (in modulo) with opposite signs, and to insufficient exploration of the neighborhoods of the vertical asymptote. Thus if a NAN is encountered during function evaluation inside the integration domain, the calculation is stopped by caution. On the other hand, if divergences occur at boundaries but the integrand function has finite limit there, the algorithm proved to able to estimate the integral. In these cases JEMDI completes the calculation but returns a warning to inform the user that the result will have some significance only if the primitive is known to have finite limit on the problematic boundary.

A third control is performed directly on the final result. The algorithm checks if the condition $\delta E_{stat}/E << 1$ is fulfilled. If it is not, a warning is printed to inform the user that the systematic error can be relevant (see section 2.4 of the main text) and it is recommended to repeat the calculation by increasing the number of trajectories, $N_{tr}$, and/or the length of the trajectories, $N_{\text{steps}}$.

## 2. Sectioned contours of function in Eq. 13 of the main text

We show in Figure 1 some sectioned contours of the 3-variables building block $\phi_A(x_{1,i}, x_{2,i}, x_{3,i})$ given in equation 13 of the main text.

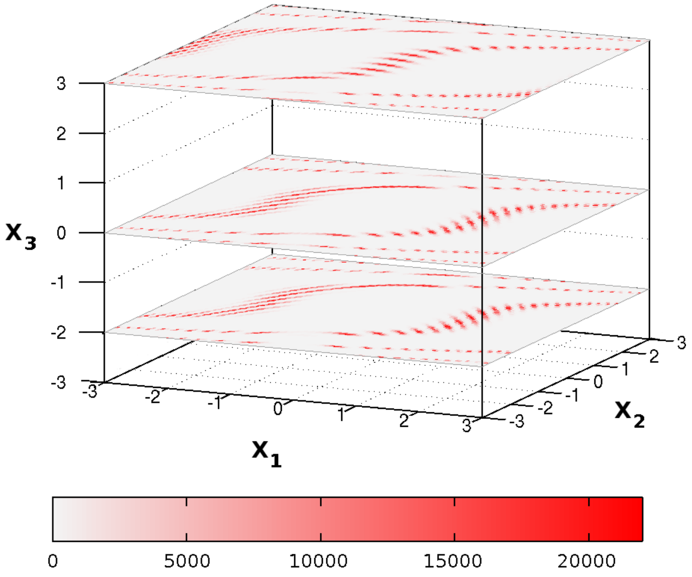


Figure 1: Selected sections at $x_3$=-2, 0, and 3 of the function $\phi_A(x_1, x_2, x_3)$. The colorbar shows that the function features large flat areas (in light gray) and clusters of tight peaks (in red).

## 3. Insight on the morphing with Monte Carlo propagator

Let us consider again the positive-valued test function illustrated in Section 2 above, generated by products of the building blocks $\phi_A(x_{1,i}, x_{2,i}, x_{3,i})$.

Here we focus on the exploration of the integration domain (boundaries from -3 to +3 for all variables) via IS-MC. At any step during function morphing, from the ensemble of $N_{tr} = 5000$ trajectories we evaluate the percentage of accepted moves, $\%_{\mathrm{acc}}$:

$$\%_{\mathrm{acc}}(s) = 100 \times \frac{1}{N_{tr}} \sum_{i=1}^{N_{tr}} \alpha(i,s) \tag{2}$$

where $s = 1, 2, ..., N_{\mathrm{steps}}$ is an integer index corresponding to the actual MC step, and $\alpha(i,s)$ is equal to 1 if for the $i$-th trajectory the attempted move at step $s$ is accepted, 0 if it is rejected. Then, by averaging the values $\%_{\mathrm{acc}}$ *up to* a given MC step, we get the average acceptance percentage $\overline{\%_{\mathrm{acc}}}$:

$$\overline{\%_{\mathrm{acc}}}(s) = \frac{1}{s} \sum_{s'=1}^{s} \%_{\mathrm{acc}}(s') \tag{3}$$

In Figures 2a,b we show, respectively, the profiles of $\overline{\%_{\mathrm{acc}}}$ and $\%_{\mathrm{acc}}$ for several values of the maximum length $\delta_{max}$ of the MC moves (here we fix $\delta_{\mathrm{max},i} \equiv \delta_{\mathrm{max}}$ for all variables). A total number of $N_{\mathrm{steps}} = 10^5$ has been performed in the morphing schedule.

Profiles start from 100% since all moves over the initial flat "potential" are clearly accepted (see equation 4 of the main text for the concept of pseudo-potential associated to the integrand function). The decrease as the morphing proceeds is due to the fact that an IS-MC path falls likely in a deep potential well, once it is developed, and remains "entrapped" in it (further moves are mostly rejected); we shall come back to this issue in the following. Such a trend is frequently expected regardless of the peculiarities of the integrand function. Apart of these expected features, the details of the profiles, for a given total number of steps (i.e., a given "speed" of morphing), are hardly predictable since they depend in subtle way on the details of the landscape of the "potential" which develops during the morphing. A case-specific knowledge previously gained would address one to "deterministically tune" the change of each $\delta_{\mathrm{max},i}$ during the morphing in order to keep $\%_{\mathrm{acc}}(s)$

as close as possible to 50%. Clearly this is a hard task, so that the rough but unbiased choice here pursued is to focus on the average $\overline{\%_{\rm acc}}$ as global indicator.

As further feature, we have explored the dependence of $\%_{\rm acc}(s)$ on $\delta_{\rm max}$ and number of variables $N$. By generating IS-MC paths for different values of these parameters, we have obtained the profiles shown in Figure 3a, where it has been chosen $s = N_{\rm steps} = 10^5$ at the end of the morphing protocol. What emerges is a power-law dependence $p_{\rm acc}(s) \sim N^{\phi(\delta_{\rm max},s)}$ for the frequency of move acceptance ($p_{\rm acc}(s) = \%_{\rm acc}(s)/100$), with $\phi(\delta_{\rm max}, s)$ a characteristic function which regulates the slope of the straight lines in the double-logarithmic diagram. The plot of $\phi(\delta_{\rm max}, s)$ versus $\delta_{\rm max}$ is presented in Figure 3b. The global message is that the optimal values $\delta_{{\rm max},i}$ which should yield an average $\overline{\%_{\rm acc}}$ close to 50% depend also, in some rather complex way, on the dimensionality of the problem ($N$) and they have to be determined case-by-case. The features displayed in Figure 3, in fact, are strictly pertinent to the specific kind of function (i.e., factorized into building blocks of the kind $\phi_A$) and integration boundaries. We recall the JEMDI routine makes automatically the search of the optimal values $\delta_{{\rm max},i}$ as described in the first part of this document.

The "entrapping" of the IS-MC paths in potential wells is revealed in Figure 4 for the case $N = 30$ variables, where the Euclidean displacement from an initial point (here we take the same point $\mathbf{x}_0$ of the profiles of Figure **??**) settles on a plateau as the morphing proceeds. Notice how the features of the profiles are strongly regulated by $\delta_{\rm max}$. For the optimal value $\delta_{\rm max} = 0.03$, which gives best estimate of the integral, the path approaches quickly a potential well and keeps an erratic behavior with large fluctuations during the whole morphing. The same initial jump occurs for the large $\delta_{\rm max} = 0.3$ but the potential well is less explored. For the smaller value $\delta_{\rm max} = 0.003$, the growth is smoother and displays low-amplitude fluctuations; this suggests that irrelevant regions are sampled during a large portion of the morphing, and that relevant potential wells (peaks of the function) are poorly explored.

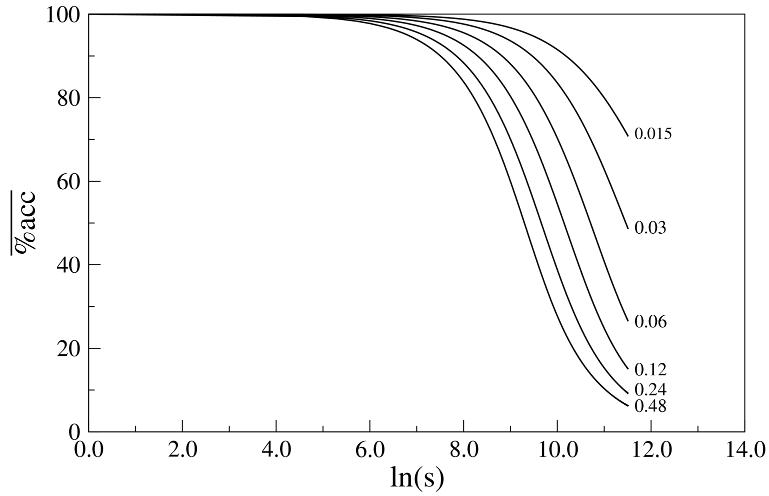


**(a)**

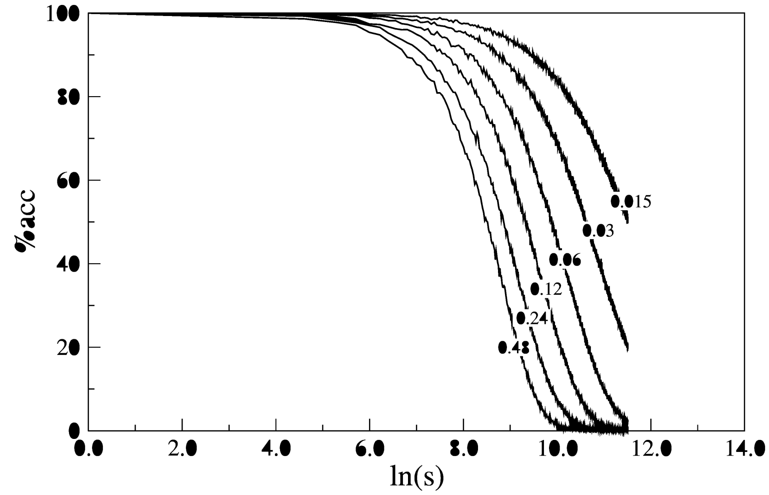


**(b)**

Figure 2: (a) Average IS-MC moves acceptance, $\overline{\%_{\text{acc}}}$, as function of the natural logarithm of the number of steps, $s$, from 1 to $N_{\text{steps}} = 10^5$. Calculations have been conducted for different values of the $\delta_{\max}$ (indicated in the plot) and $N_{tr} = 5000$. The integrand function is generated as product of building blocks $\phi_A$ with $N = 30$ variables. (b) IS-MC moves acceptance $\%_{\text{acc}}$ as function of the natural logarithm of the number of steps, $s$ obtained from the same calculation.

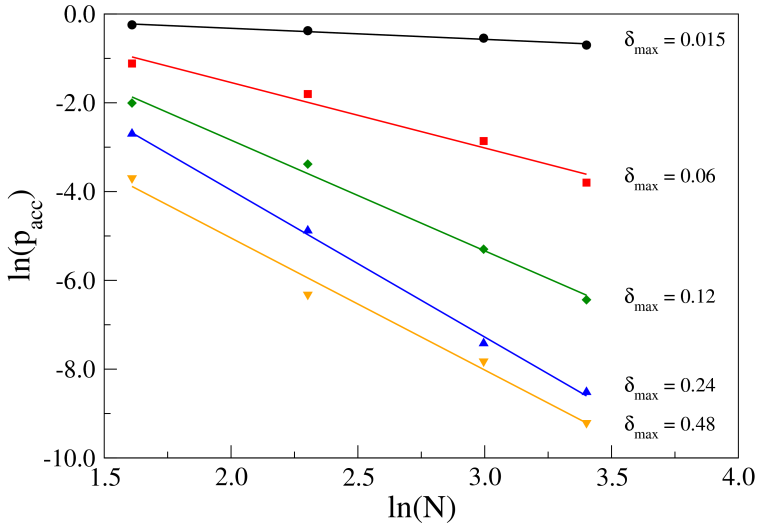


**(a)**

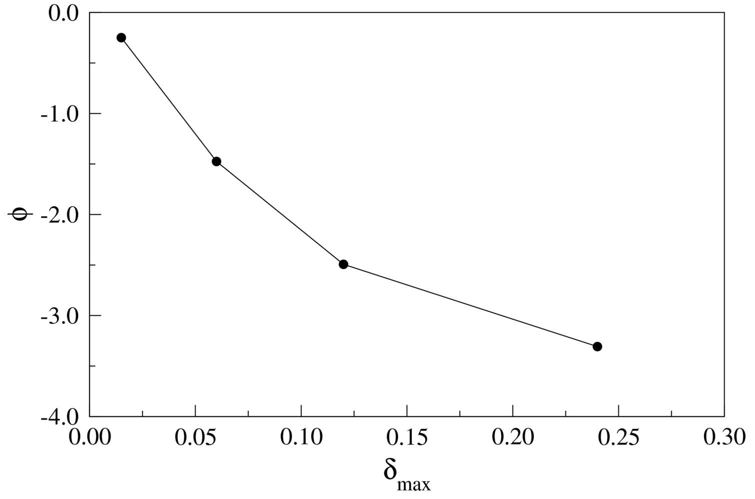


**(b)**

Figure 3: (a) Natural logarithm of $p_{acc} = \%_{\mathrm{acc}}/100$ as function of the natural logarithm of the number of variables for different values of $\delta_{\mathrm{max}}$ (indicated in the plot), at the last step of morphing ($s = N_{\mathrm{steps}} = 10^5$). $N_{tr} = 5000$ IS-MC trajectories have been generated. The integrand function is generated as product of building blocks $\phi_A$ with $N = 30$ variables. Straight lines have been obtained from the linear regression of the data. (b) Profiles of the slope $\phi(\delta_{\mathrm{max}}, s)$ as function of $\delta_{\mathrm{max}}$ from fits of the points in the left panel (the value at $\delta_{\mathrm{max}} = 0.48$ is excluded because of too large uncertainty).

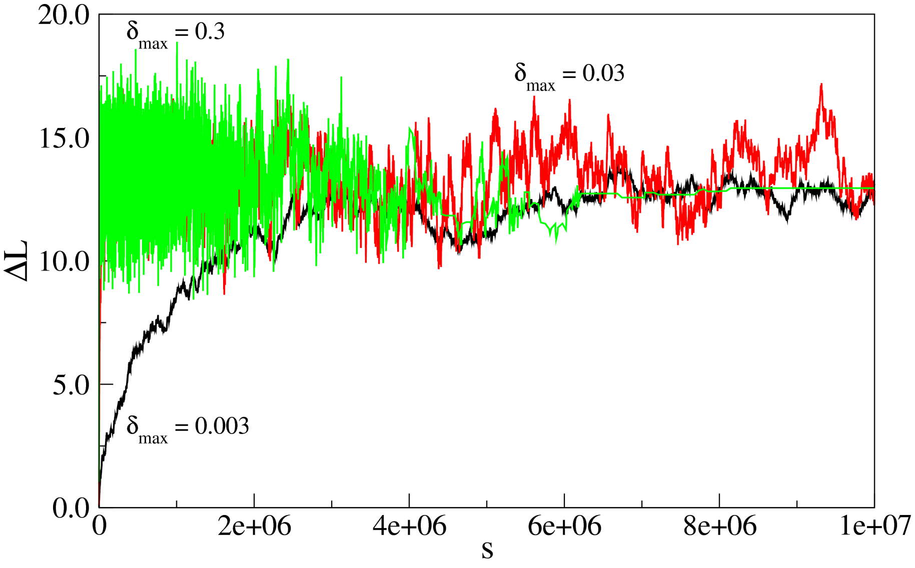


Figure 4: Plot of the Euclidean displacement $\Delta L$ vs. the number of IS-MC trajectory steps for three values of $\delta_{\max}$, i.e 0.003 (black line), 0.03 (red line), 0.3 (green line). In the three calculations, $\Delta L$ has been evaluated with respect to the same initial point $\boldsymbol{x}_0$. The integrand function is generated as product of building blocks $\phi_A$ with $N = 30$ variables. Morphing was done with $N_{\text{steps}} = 10^7$.

## References

[1] W. H. Press, S. A. Teukolsky, W. T. Vetterling, B. P. Flannery, Numerical Recipes in C: The Art of Scientific Computing, Cambridge University Press, New York, 1992.

[2] M. Mascagni, A. Srinivasan, ACM Trans. Math. Softw. 26 (2000) 436-461.

[3] A. Srinivasan, M. Mascagni, D. Ceperley, Parallel Comput. 29 (2003) 68-84.

[4] J. R. Michael, W. R. Schucany, R. W. Haas, The American Statistician 30 (1976) 88-90.

[5] G. Box, M. E. Muller, Ann. Math. Stat. 29 (1958) 610-611.

[6] M. C. Jeruchim, P. Balaban, K. S. Shanmugan, Simulation of communication systems, Plenum Press, New York, 1992.
